# Supplementary material for: DOM-Q-NET: Grounded RL on Structured Language
Source: arXiv:1902.07257 source file (2019-02-19)

# Goal Attention Readout Phase

$$h_{global} = \sum_{i=1}^V \alpha_i h_i^T$$

$$\alpha_i = \frac{h_i^0 \cdot h_{goal}}{\sum_{j=1}^V h_j^0 \cdot h_{goal}}$$

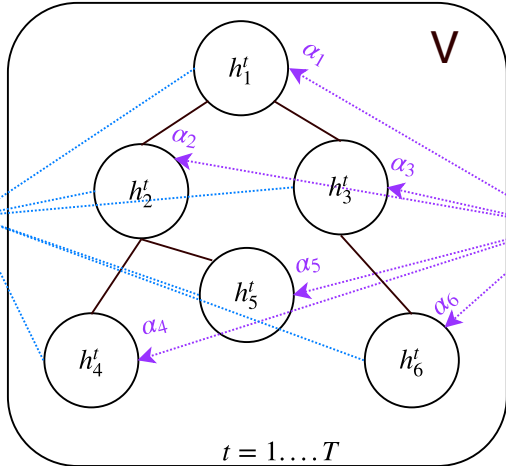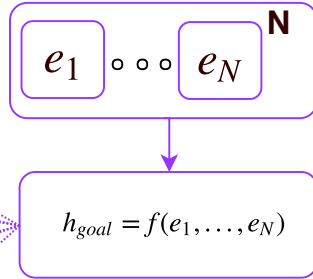

Supplement: Supplementary file 1 [file ga_diag.pdf]
