# Supplementary material for: DOM-Q-NET: Grounded RL on Structured Language
Source: arXiv:1902.07257 source file (2019-02-19)

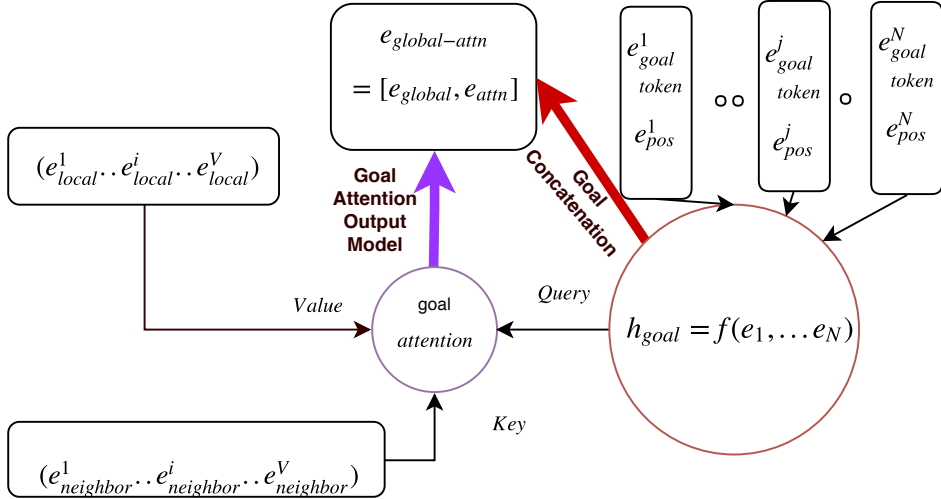

Supplement: Supplementary file 2 [file goal_encoder.pdf]
